# Supplementary material for: Volume Conductor: Interactive Visibility Management for Crowded Volumes
Source: arXiv:2206.07392 source file (2022-06-15)
Supplement: Supplementary file 1 [file supplementary.tex]

\section*{Supplemental Material}

\subsection*{Additional performance analysis results}

In \cref{tab:performance}, we list the timing for all three evaluated steps (linearization and shader recompilation, visibility mask computation, and rendering) for all graphics cards on all the datasets. On the Nvidia Quadro RTX 8000,  the DOS method still runs at around 2 frames per second (FPS) at a $2048 \times 2048$ resolution with 1024 slices, and at 4 to 7 FPS at a $1024 \times 1024$ resolution with 512 slices even for the largest datasets (fibers and mitochondria).

\begin{table}[!htb]
    \centering
    \scriptsize
    \begin{tabularx}{\linewidth}{X|c|c|c|c|}
        & \textbf{Frame size} & \multicolumn{3}{c|}{\textbf{Number of slices}} \\
        &            & 256 & 512 & 1024 \\ \hline\hline
        \multicolumn{5}{c}{\textbf{Integrated graphics}} \\ \hline
        \multirow{3}{*}{\rotatebox[origin=c]{90}{\textbf{Fibers}}}
        & $512 \times 512$   & 6 / 468 / 429 & 5 / 468 / 786 & 6 / 468 / 1502 \\
        & $1024 \times 1024$ & 6 / 469 / 1012 & 7 / 468 / 1917 & 6 / 468 / 3722 \\
        & $2048 \times 2048$ & 9 / 471 / 2736 & 10 / 471 / 5210 & 9 / 472 / 10170 \\ \hline
        \multirow{3}{*}{\rotatebox[origin=c]{90}{\textbf{Pores}}}
        & $512 \times 512$   & 5 / 545 / 464 & 6 / 556 / 839 & 5 / 545 / 1629 \\
        & $1024 \times 1024$ & 6 / 533 / 934 & 7 / 535 / 1760 & 6 / 542 / 3439 \\
        & $2048 \times 2048$ & 9 / 551 / 2618 & 8 / 551 / 4990 & 9 / 545 / 9772 \\ \hline
        \multirow{3}{*}{\rotatebox[origin=c]{90}{\textbf{Mitos}}}
        & $512 \times 512$   & 6 / 546 / 487 & 6 / 545 / 898 & 5 / 546 / 1734 \\
        & $1024 \times 1024$ & 5 / 547 / 985 & 7 / 546 / 1839 & 6 / 545 / 3655 \\
        & $2048 \times 2048$ & 8 / 550 / 2642 & 8 / 552 / 5036 & 8 / 548 / 9825 \\ \hline\hline
        \multicolumn{5}{c}{\textbf{Commodity desktop graphics}} \\ \hline
        \multirow{3}{*}{\rotatebox[origin=c]{90}{\textbf{Fibers}}}
        & $512 \times 512$   & 9 / 89 / 221 & 11 / 89 / 421 & 15 / 89 / 805 \\
        & $1024 \times 1024$ & 12 / 89 / 215 & 15 / 89 / 373 & 12 / 89 / 689 \\
        & $2048 \times 2048$ & 14 / 89 / 405 & 15 / 89 / 617 & 13 / 89 / 1203 \\ \hline
        \multirow{3}{*}{\rotatebox[origin=c]{90}{\textbf{Pores}}}
        & $512 \times 512$   & 7 / 56 / 161 & 15 / 47 / 287 & 18 / 52 / 542 \\
        & $1024 \times 1024$ & 21 / 48 / 172 & 12 / 52 / 294 & 19 / 50 / 523 \\
        & $2048 \times 2048$ & 13 / 48 / 356 & 15 / 48 / 597 & 15 / 49 / 1068 \\ \hline
        \multirow{3}{*}{\rotatebox[origin=c]{90}{\textbf{Mitos}}}
        & $512 \times 512$   & 9 / 26 / 101 & 9 / 29 / 187 & 11 / 27 / 327 \\
        & $1024 \times 1024$ & 9 / 27 / 134 & 12 / 27 / 215 & 15 / 27 / 383 \\
        & $2048 \times 2048$ & 17 / 27 / 340 & 17 / 27 / 575 & 18 / 29 / 1018 \\ \hline\hline
        \multicolumn{5}{c}{\textbf{Professional graphics}} \\ \hline
        \multirow{3}{*}{\rotatebox[origin=c]{90}{\textbf{Fibers}}}
        & $512 \times 512$   & 5 / 85 / 34 & 7 / 85 / 55 & 5 / 85 / 100 \\
        & $1024 \times 1024$ & 5 / 85 / 81 & 5 / 85 / 138 & 4 / 85 / 248 \\
        & $2048 \times 2048$ & 4 / 86 / 204 & 4 / 87 / 324 & 4 / 91 / 580 \\ \hline
        \multirow{3}{*}{\rotatebox[origin=c]{90}{\textbf{Pores}}}
        & $512 \times 512$   & 5 / 47 / 26 & 5 / 47 / 41 & 4 / 47 / 72 \\
        & $1024 \times 1024$ & 4 / 47 / 60 & 4 / 46 / 92 & 4 / 46 / 156 \\
        & $2048 \times 2048$ & 4 / 46 / 162 & 4 / 46 / 231 & 4 / 50 / 368 \\ \hline
        \multirow{3}{*}{\rotatebox[origin=c]{90}{\textbf{Mitos}}}
        & $512 \times 512$   & 5 / 26 / 39 & 6 / 26 / 67 & 5 / 25 / 123 \\
        & $1024 \times 1024$ & 4 / 25 / 91 & 4 / 25 / 160 & 4 / 25 / 294 \\
        & $2048 \times 2048$ & 4 / 25 / 203 & 4 / 25 / 326 & 4 / 25 / 574 \\ \hline\hline
    \end{tabularx}
    \caption{Performance evaluation of the volume conductor. The three numbers are the times in milliseconds to linearize the predicates and recompile the shader, recompute the visibility mask, and render the image.}
    \label{tab:performance}
\end{table}

We also present additional graphs for commodity desktop graphics (\cref{fig:resultsGraph2}) and professional graphics (\cref{fig:resultsGraph3}).

\begin{figure}[!hbtp]
	\centering
	\includegraphics[width=\linewidth, trim=0 0 0 1.5cm, clip]{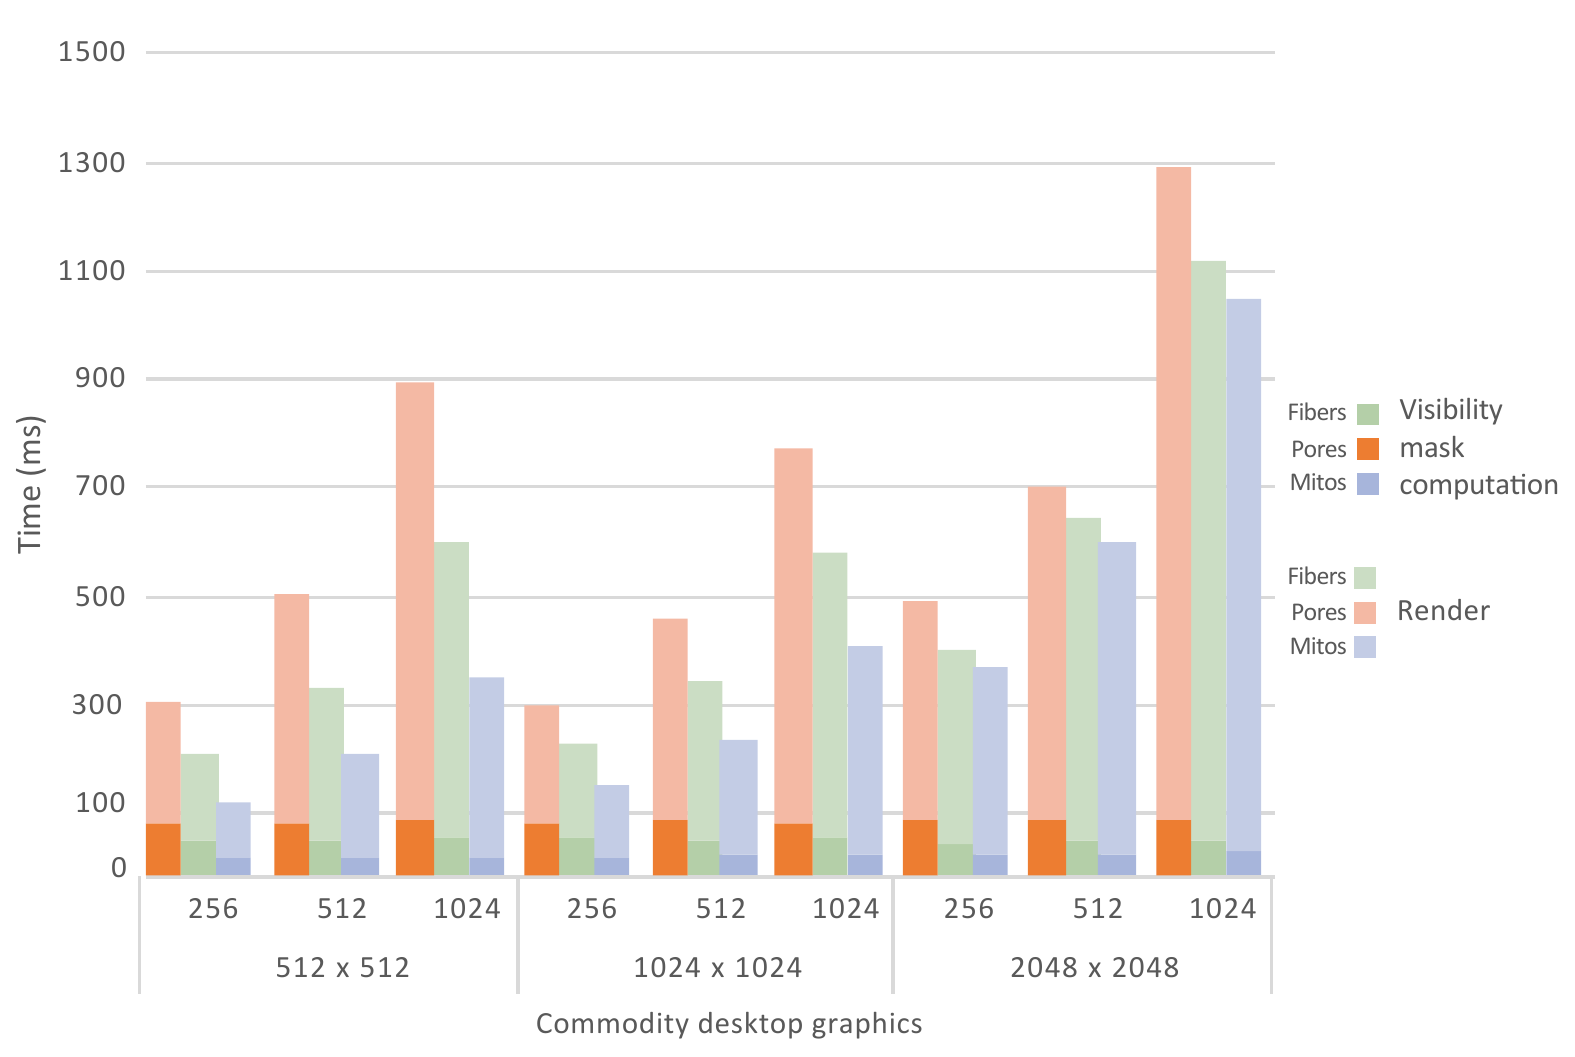}
	\caption{Performance evaluation for three datasets: fibers, pores, and mitochondria on a commodity desktop computer with an Nvidia GTX 1060 graphics card.}
	\label{fig:resultsGraph2}
\end{figure}

\begin{figure}[!hbtp]
	\centering
	\includegraphics[width=\linewidth, trim=0 0 0 1cm, clip]{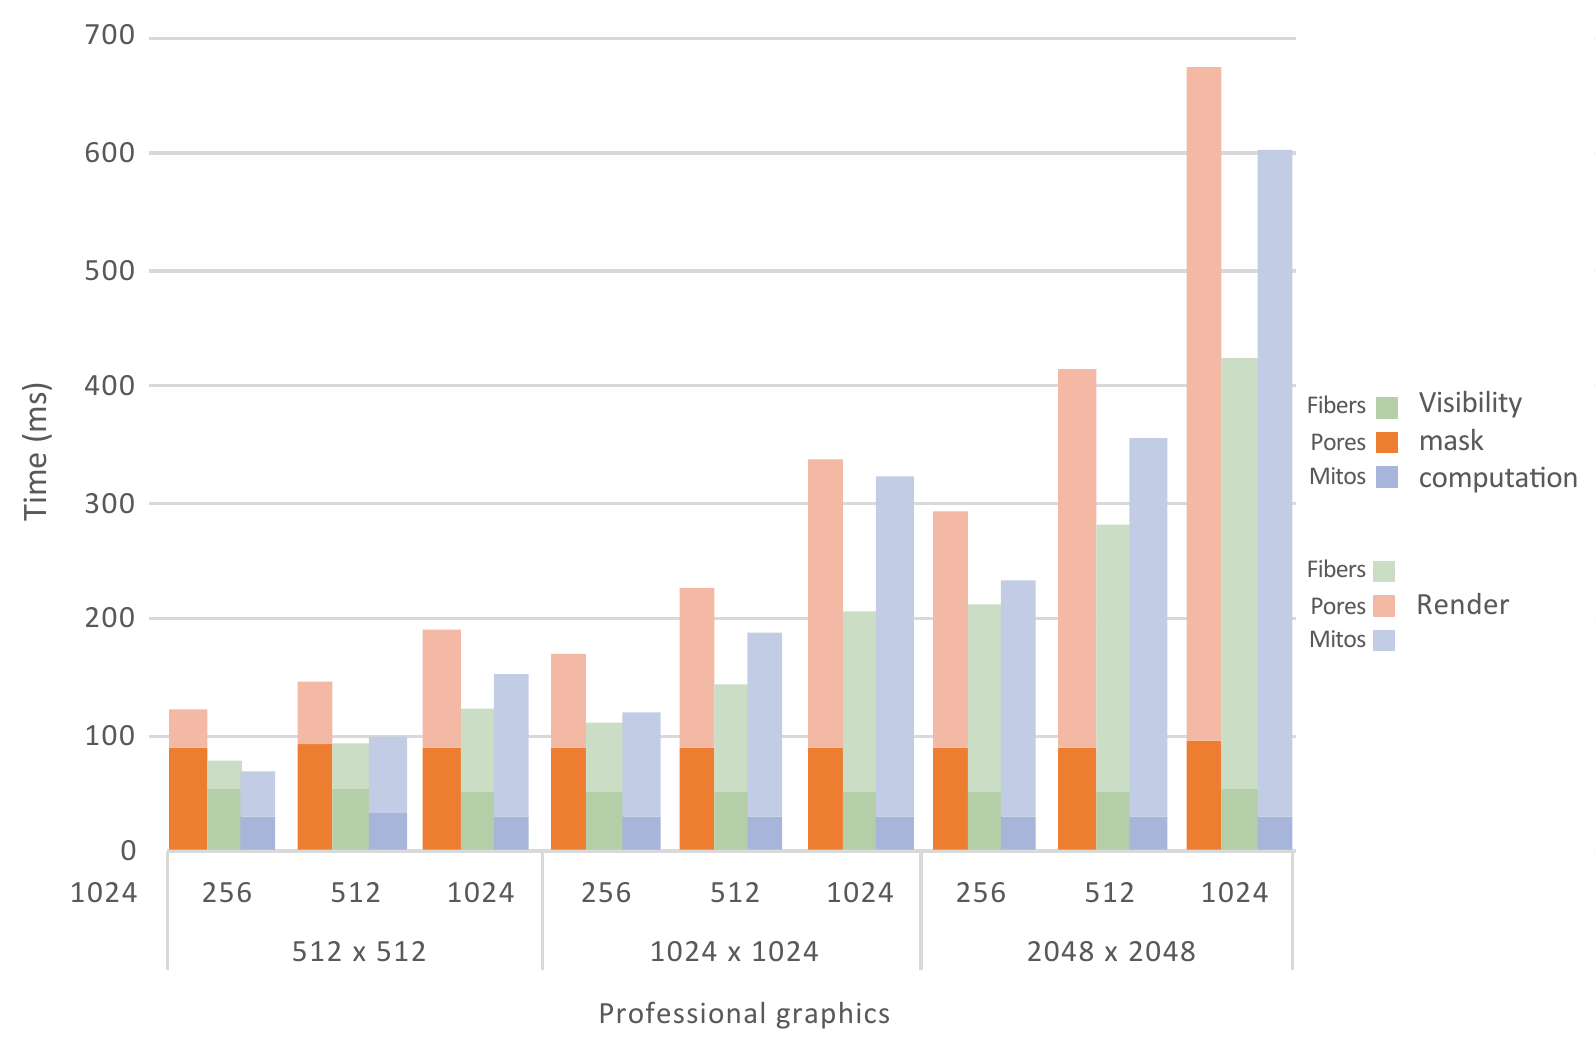}
	\caption{Performance evaluation for three datasets: fibers, pores, and mitochondria on a professional workstation with an Nvidia Quadro RTX 8000 graphics card.}
	\label{fig:resultsGraph3}
\end{figure}

\subsection*{Algorithms}

Algorithms \cref{alg:sparsification} and \cref{alg:visibility-mask} describe the instance sparsification and visibility mask generation processes in detail.

\subsection*{Online repository and examples}

The source code and all examples with synthetic data are available online at \url{http://lgm.fri.uni-lj.si/portfolio-view/volume-conductor}. The online demo is implemented in WebGL 2.0 Compute. While the API is unsupported in stable releases of web browsers, the demo can be tested in Chromium Dev build 87 available at \url{https://commondatastorage.googleapis.com/chromium-browser-snapshots/index.html}.

\subsection*{Additional examples}

This section contains additional examples of the features of the volume conductor. \cref{fig:montage} presents additional renders of the fibers, pores, and mitochondria. \cref{fig:sparsification-functions} shows the effects of different sparsification functions on a synthetic dataset. In \cref{fig:sparsification} and \cref{fig:blending-and-ghosting}, we used another synthetic dataset containing boxes, spheres, and ellipsoids of various sizes. The distribution of most instances is uniform, except for ellipsoids, which are placed along one of the spatial diagonals of the volume. A large sphere is placed in the center of the volume, which is not visible without sparsification. The volume conductor is designed to be independent of the rendering method; thus, we include a comparison of path tracing and directional occlusion shading (\cref{fig:rendering-methods}).

\begin{figure*}
    \centering
    \includegraphics[width=\linewidth]{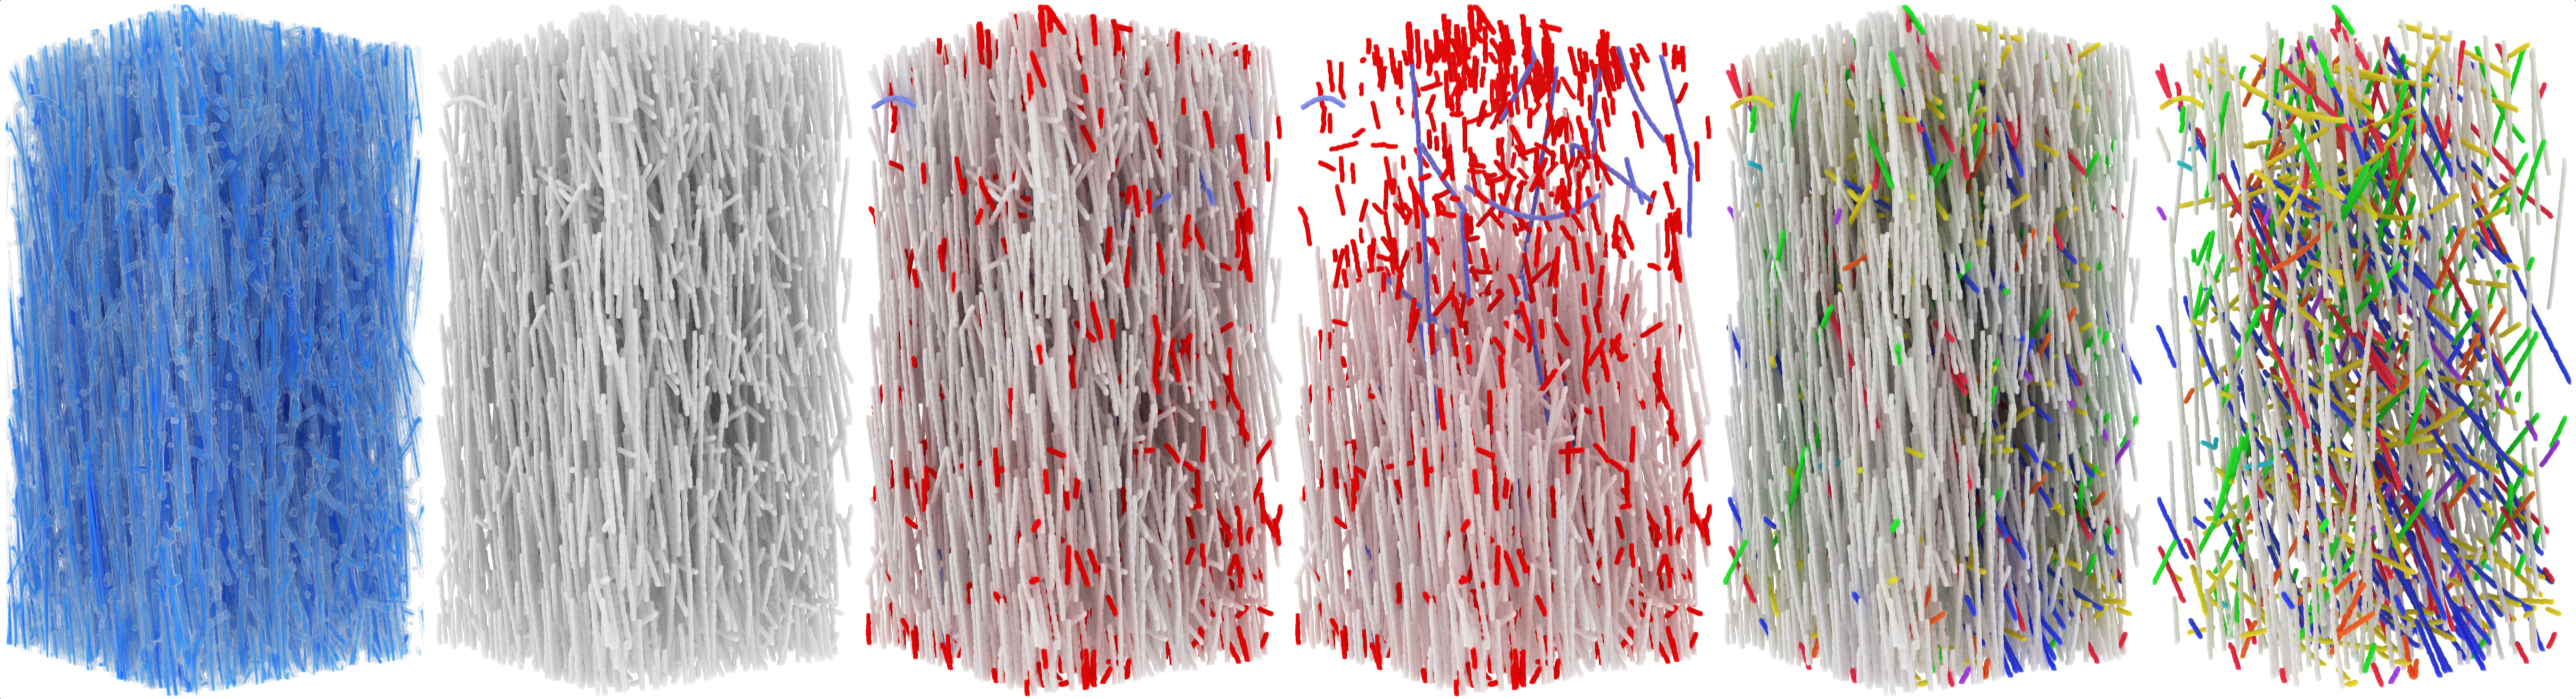}\\
    \includegraphics[width=\linewidth]{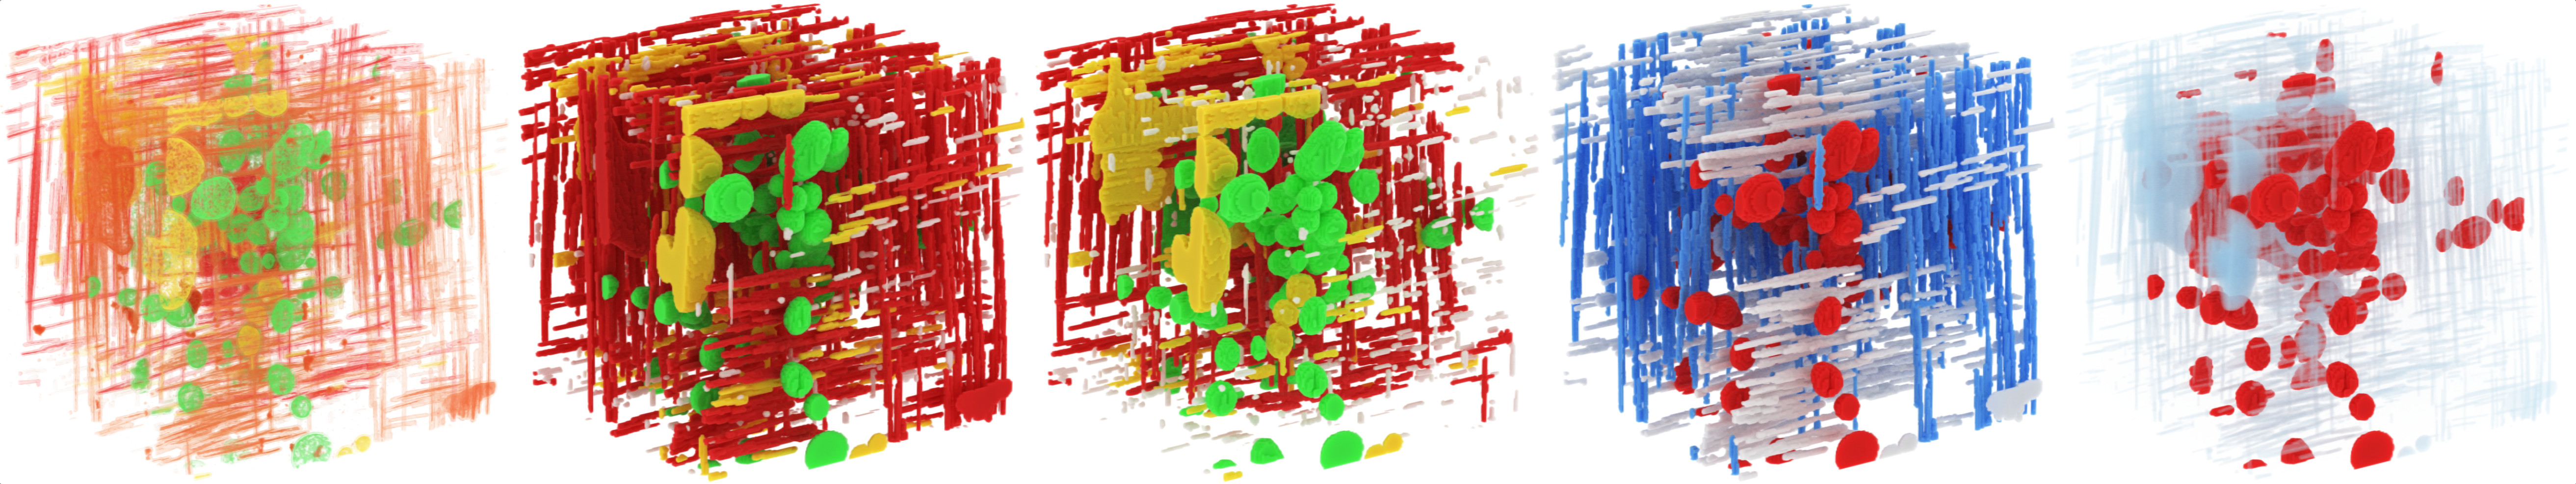}\\
    \includegraphics[width=\linewidth]{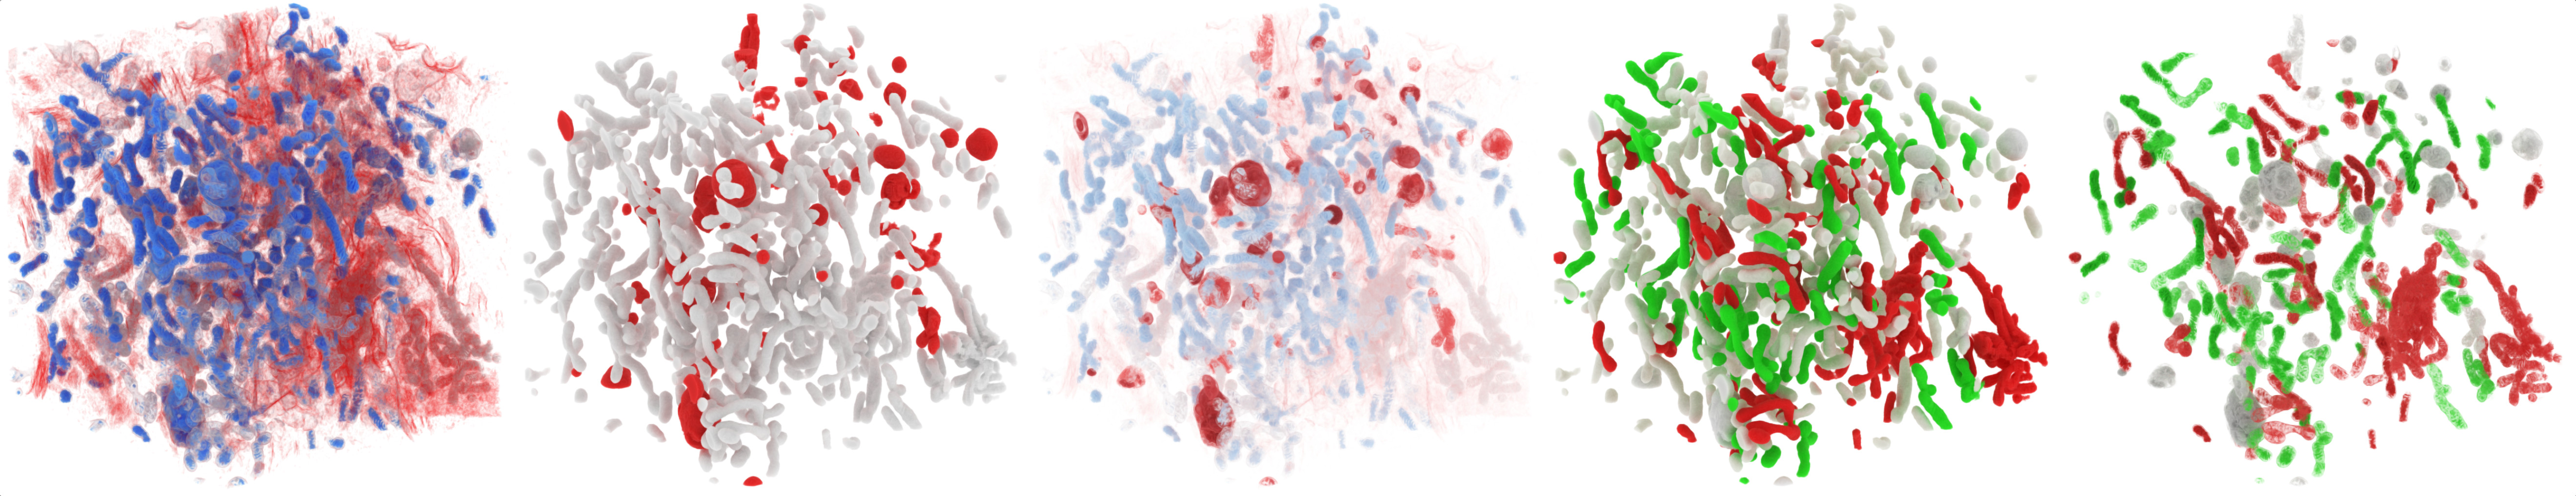}
    \caption{\textbf{Top row, fibers:} raw data, segmentation, colorization of short (red) and bent (blue) instances, same as previous but with 50~\% of the remaining instances hidden, colorization by orientation, the same as previous with 80~\% of the vertical fibers hidden. \textbf{Middle row, pores:} raw data, colorization by roundedness, the same as previous with 50~\% of the needle-shaped pores hidden, colorization of needle-shaped pores by orientation, and ghosting. \textbf{Bottom row, mitochondria:} raw data, colorization of type, the same as previous but with added blending with raw data, colorization by branching and thinning, same as previous with opacity transfer. Path tracing was used to generate the images.}
    \label{fig:montage}
\end{figure*}

\begin{algorithm}
    \begin{algorithmic}[1]
        \scriptsize
        \FORALL {$i \in \mathrm{instances}$}
            \STATE $hidden_i \gets \FALSE$
        \ENDFOR
        \FORALL {$r \in \mathrm{predicates}$}
            \STATE $G \gets \mathbf{instances}(r)$
            \STATE $n_{hidden} \gets 0$
            \STATE $n_{toHide} \gets \lfloor \mathbf{visibilityRatio}(r) \cdot |G| \rfloor$
            \STATE $\mathbf{sort}(G)$
            \FORALL {$i \in G$}
                \IF {\NOT $hidden_i$ \AND \NOT $visible_i$}
                    \STATE $n_{hidden} \gets n_{hidden} + 1$
                    \STATE $hidden_i \gets \TRUE$
                    \IF {$n_{hidden} = n_{toHide}$}
                        \STATE $\mathbf{break}$
                    \ENDIF
                \ENDIF
            \ENDFOR
            \FORALL {$i \in G$}
                \IF {$hidden_i$}
                    \STATE $\mathbf{continue}$
                \ELSIF {$n_{hidden} \leq n_{toHide}$}
                    \STATE $n_{hidden} \gets n_{hidden} + 1$
                    \STATE $visible_i \gets \FALSE$
                \ELSE
                    \STATE $visible_i \gets \TRUE$
                \ENDIF
            \ENDFOR
        \ENDFOR
    \end{algorithmic}
    \caption{Sparsification with temporal coherency.}
    \label{alg:sparsification}
\end{algorithm}

\begin{algorithm}
    \begin{algorithmic}[1]
        \scriptsize
        \FORALL {$i \in \mathrm{instances}$}
            \FORALL {$r \in \mathrm{predicates}$}
                \IF {$r(i)$}
                    \IF {$visible_i$}
                        \STATE $group_i \gets r$
                        \STATE $maskValue_i \gets \mathbf{maskValue}(r)$
                    \ELSE
                        \STATE $group_i \gets 0$
                        \STATE $maskValue_i \gets \mathbf{maskValue}(0)$
                    \ENDIF
                \ENDIF
            \ENDFOR
        \ENDFOR
        \FORALL {$v \in \mathrm{voxels}$}
            \STATE $i \gets \mathbf{id}(v)$
            \STATE $maskValue_v \gets maskValue_i$
        \ENDFOR
    \end{algorithmic}
    \caption{Visibility mask generation.}
    \label{alg:visibility-mask}
\end{algorithm}

\begin{figure*}
    \centering
    \includegraphics[width=\linewidth]{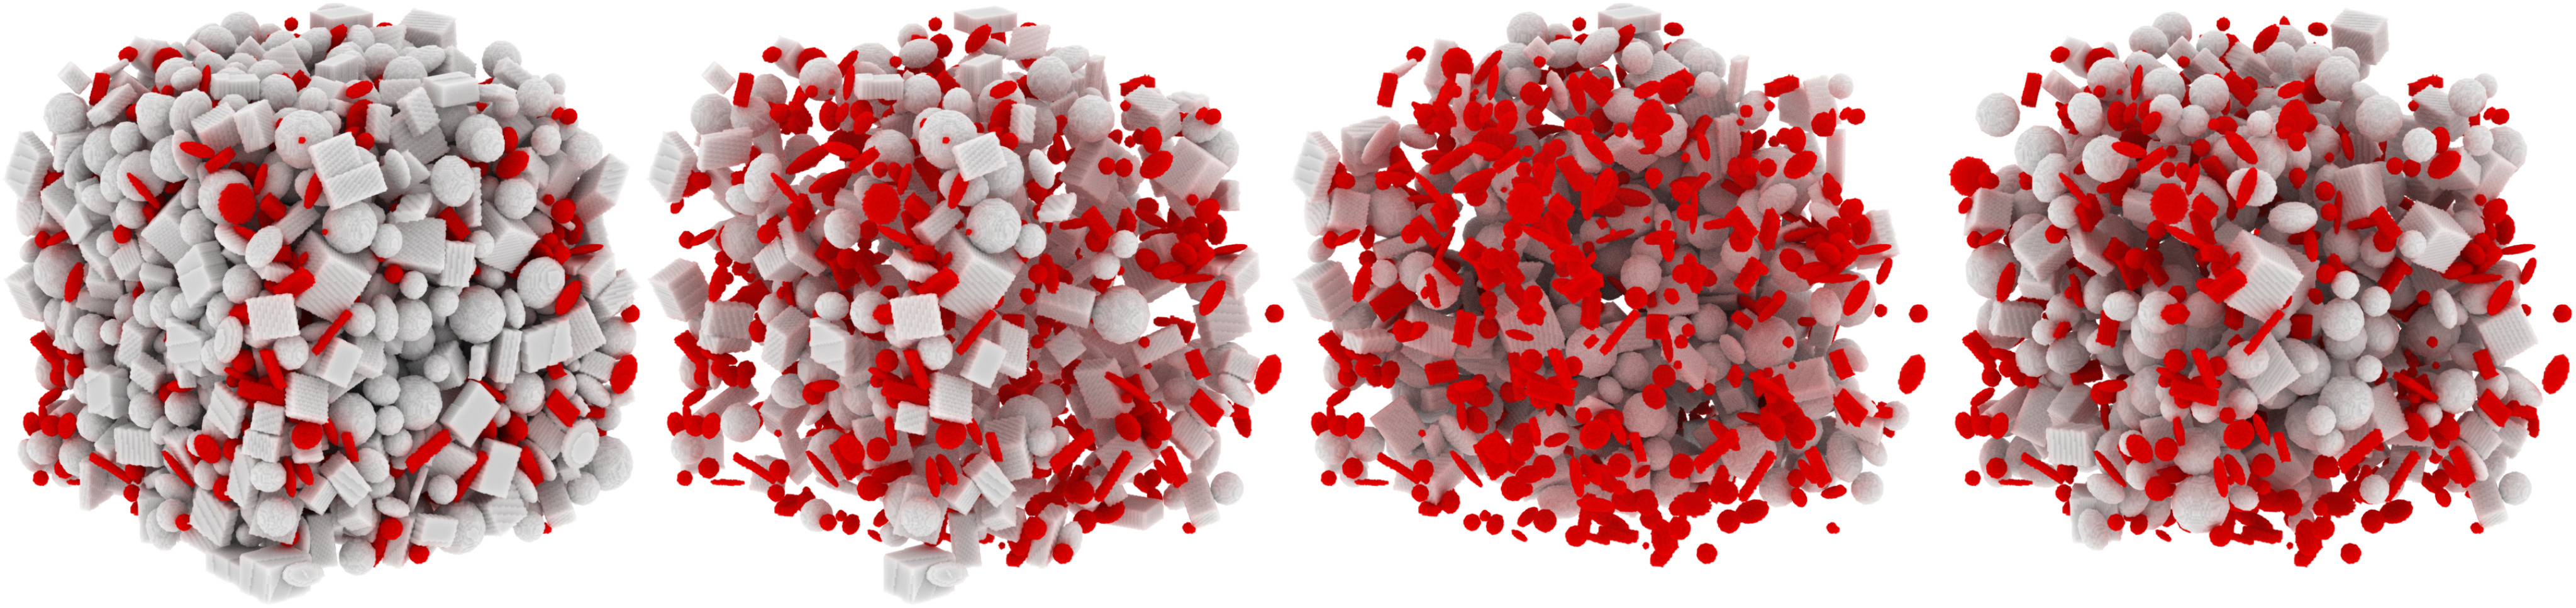}
    \caption{Demonstration of sparsification functions. From left to right: no sparsification, random, depth-based, and context-preserving sparsification. Instances with a small volume are colored red. Path tracing was used to generate the images.}
    \label{fig:sparsification-functions}
\end{figure*}

\begin{figure}
    \centering
    \includegraphics[width=\linewidth]{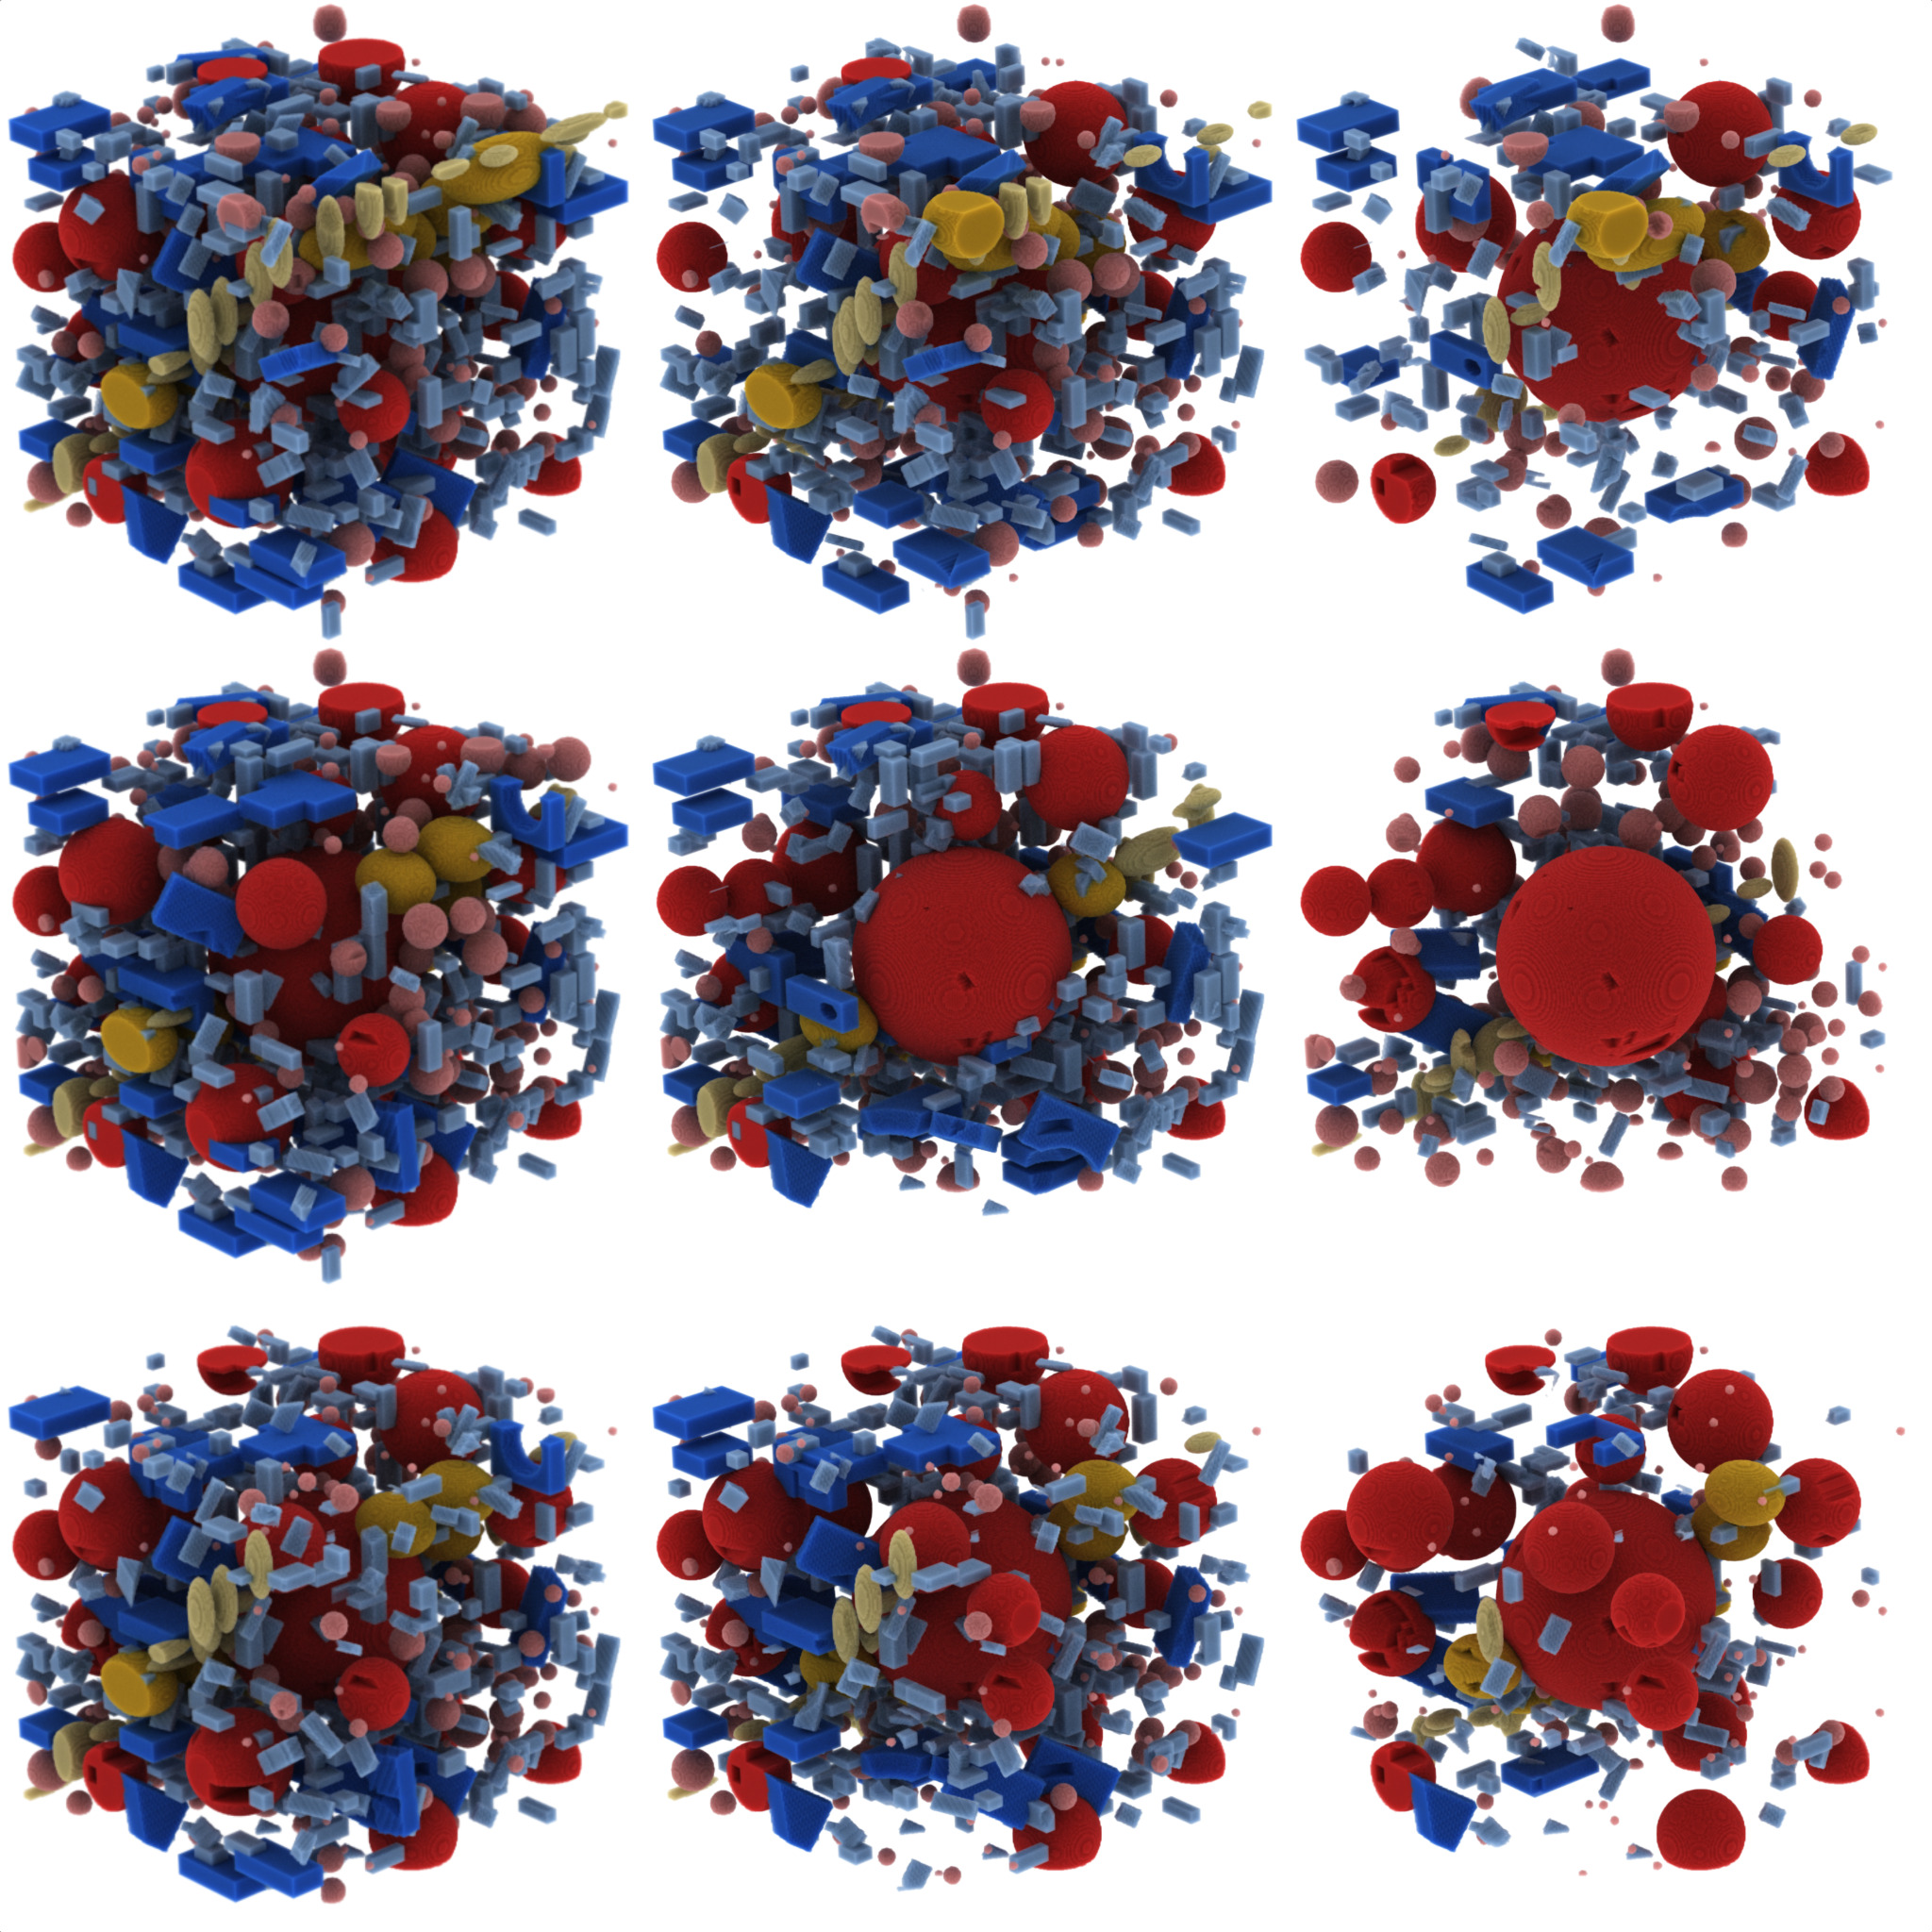}%
    \caption{From left to right: increasing degrees of uniform (top row), depth-based (middle row), and context-preserving (bottom row) sparsification.}
    \label{fig:sparsification}
\end{figure}

\begin{figure}
    \centering
    \includegraphics[width=\linewidth]{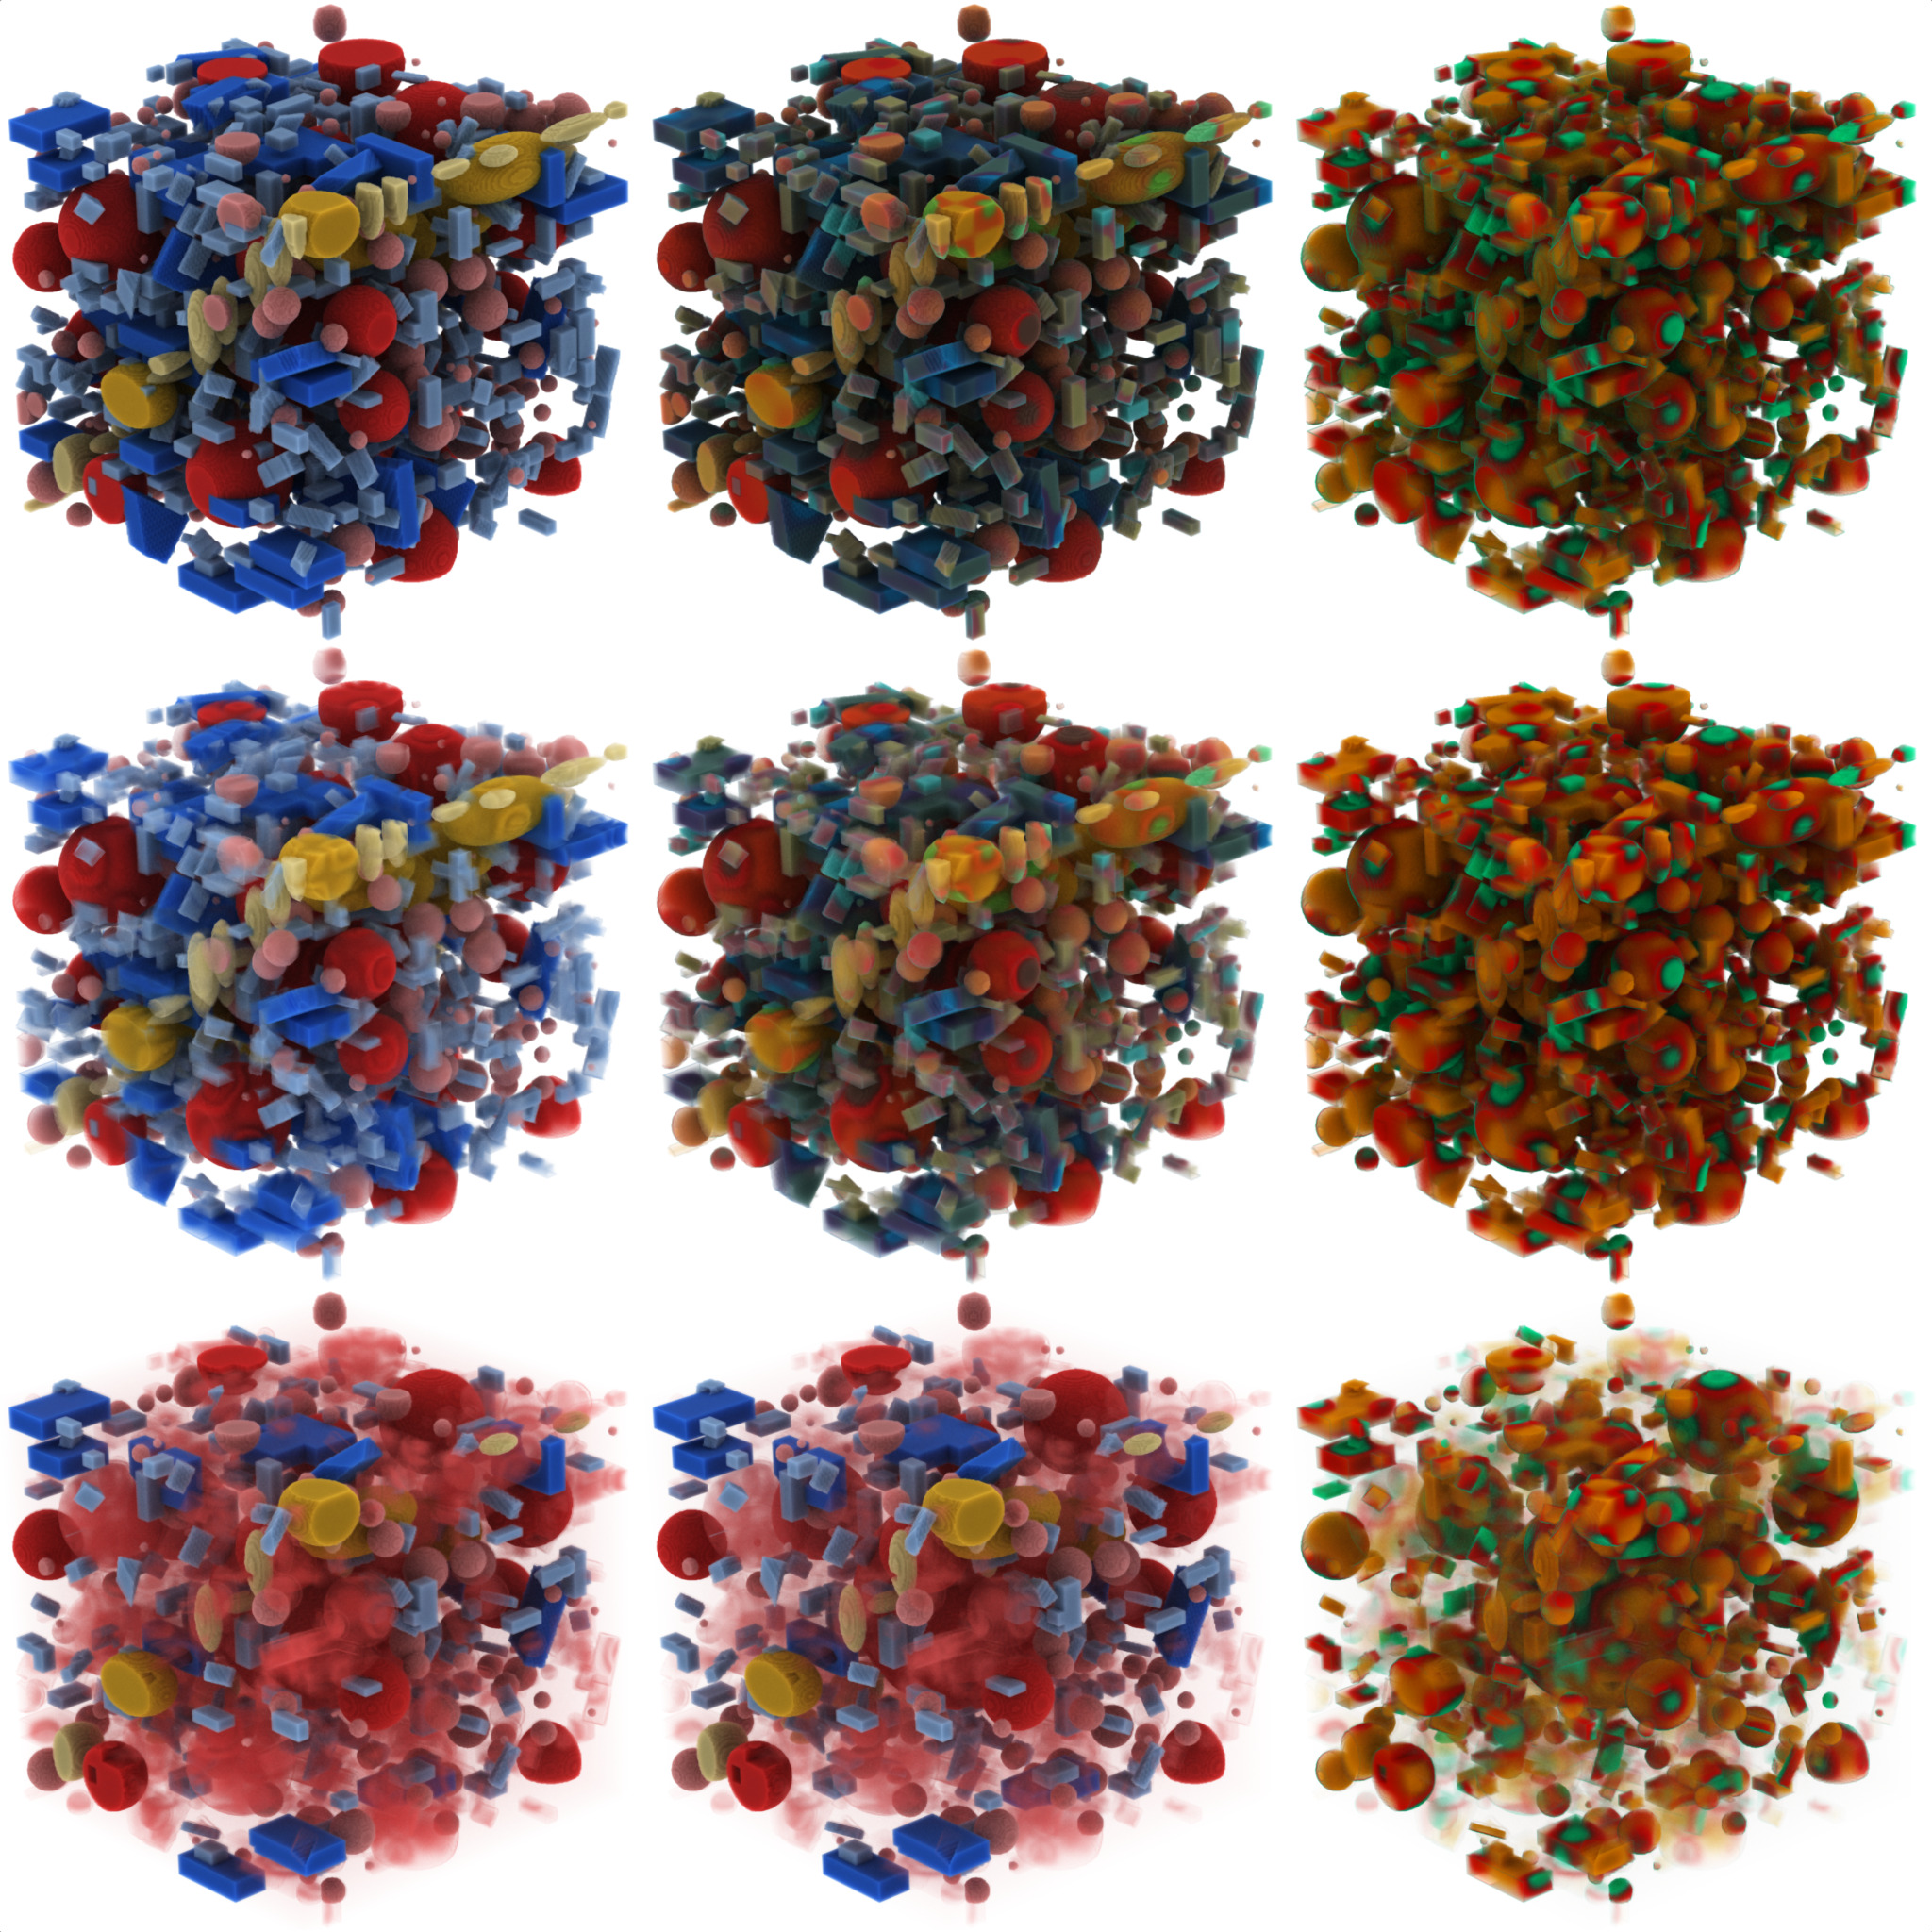}%
    \caption{Top row: different colorization as a result of blending the raw data and segmentation data transfer functions. Middle row: the same colors as above, but with the opacity transferred from the raw data transfer function, enabling the user to employ both the sparsification features of the volume conductor and the opacity set by the transfer function. Bottom row: ghosting of the instances as a result of blending the opacity after sparsification.}
    \label{fig:blending-and-ghosting}
\end{figure}

\begin{figure}
    \centering
    \includegraphics[width=\linewidth]{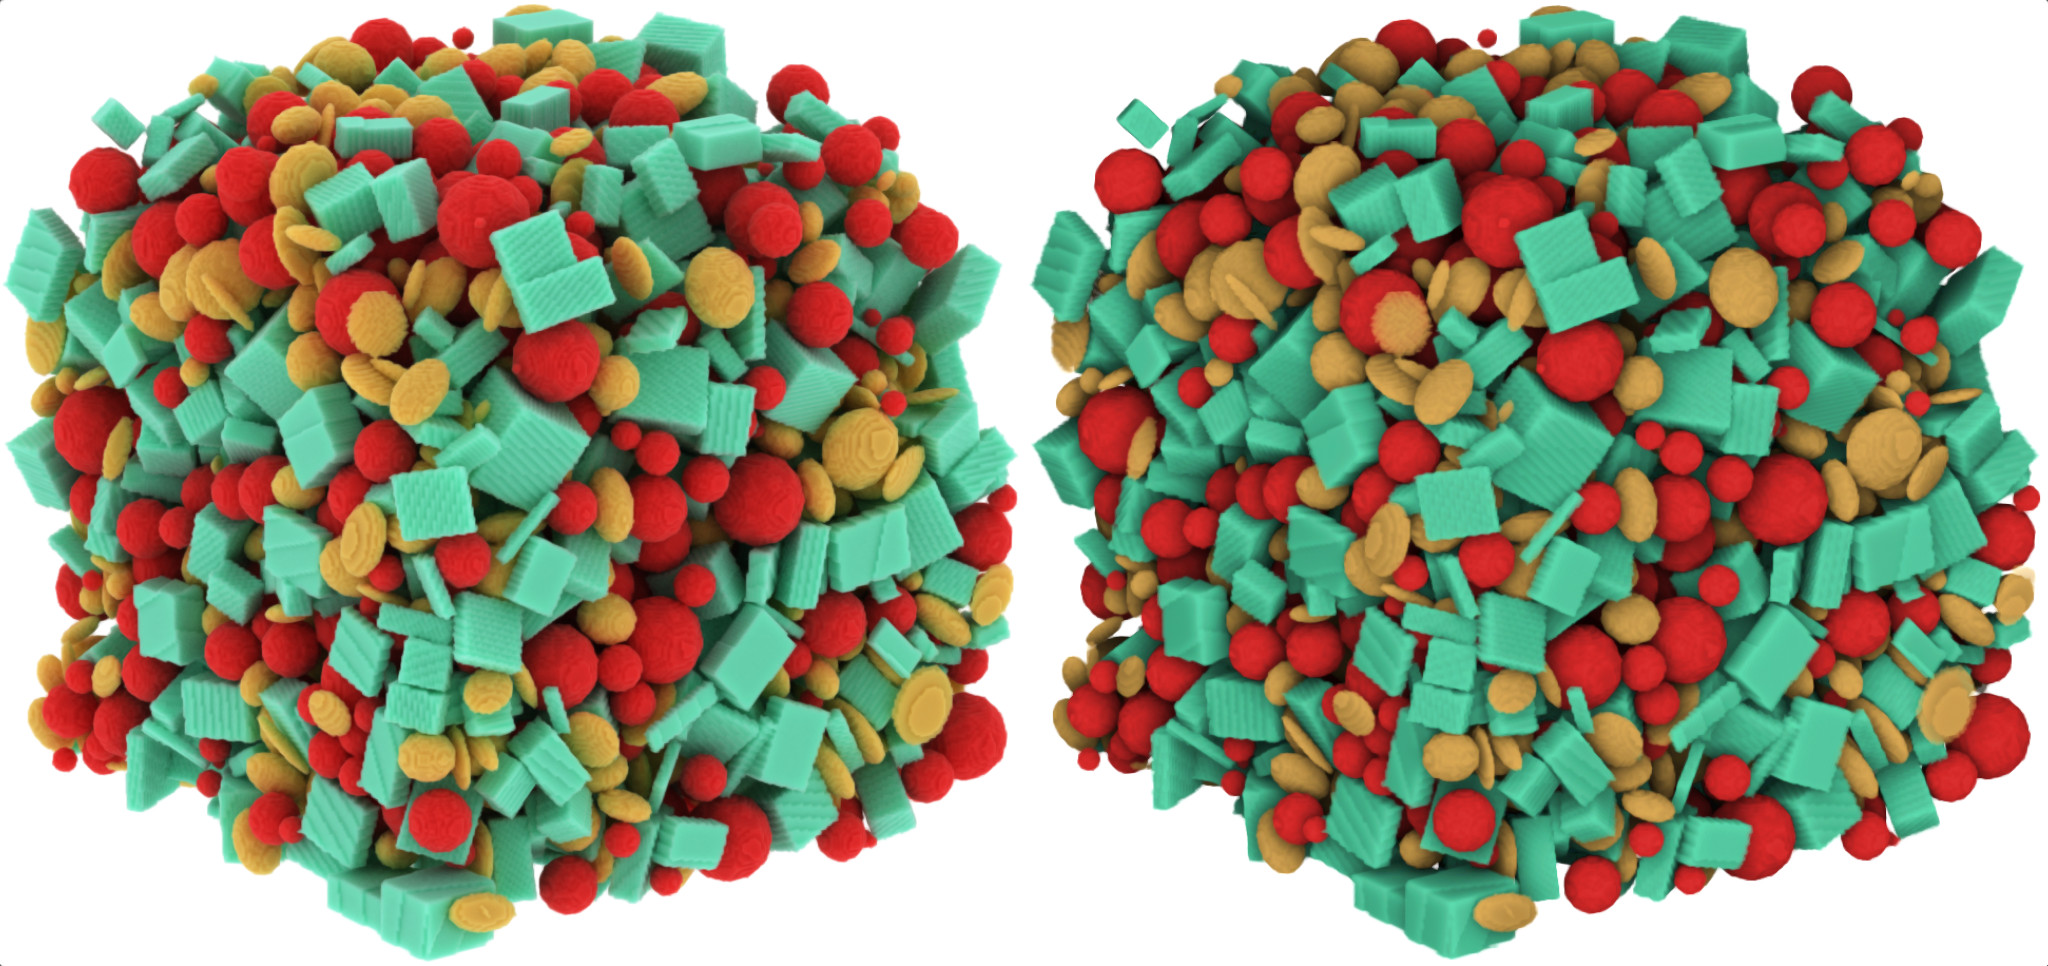}
    \caption{Left: Rendering comparison of path tracing; Right: directional occlusion shading.}
    \label{fig:rendering-methods}
\end{figure}
